# Supplementary material for: Multiple Broken Symmetries in Striped La$_{2-x}$Ba$_{x}$CuO$_{4}$ detected by the Field Symmetric Nernst Effect
Source: arXiv:1506.01994 source file (2015-06-05)

**a**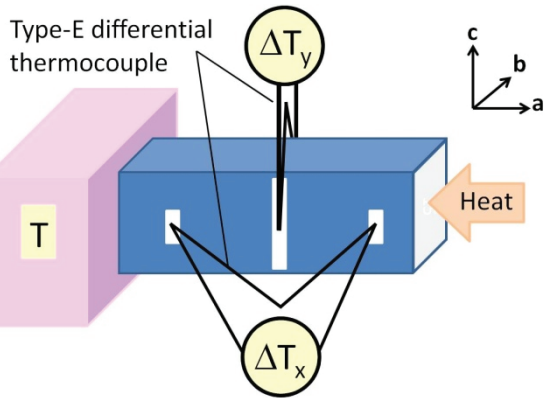**b**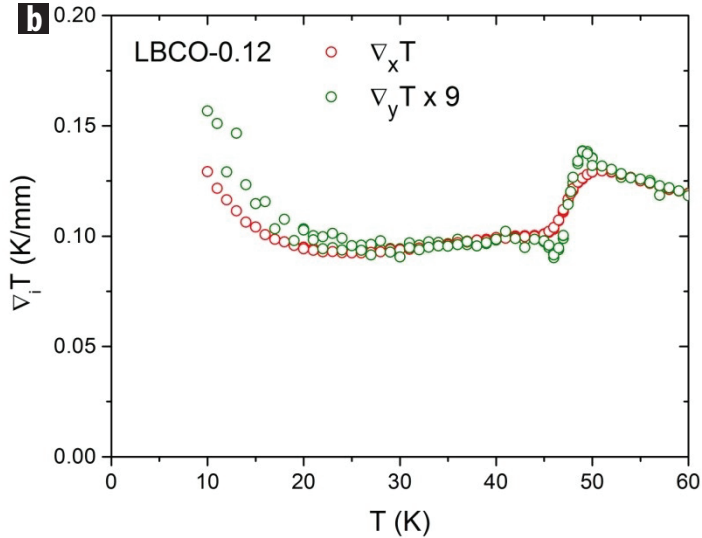

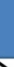

Supplement: Supplementary file 1 [file SOM_TempGrad_Meas.pdf]
